# Supplementary material for: LaSagnA: Language-based Segmentation Assistant for Complex Queries
Source: arXiv:2404.08506 source file (2024-04-12)
Supplement: Supplementary file 1 [file X_suppl.tex]

\clearpage
\setcounter{page}{1}
\maketitlesupplementary

\section{Visualization of Reconstruction}
\label{sec:viusal_recon}
We visualize the reconstructed video frames in Figure~\ref{fig:visual_recon}. We can see that the masked object areas could be regenerated through our object perception-enhanced learning.

\section{Visualization of Object Boundaries}
\label{sec:visual_bound}
We visualize the multi-scale object boundaries in Figure~\ref{fig:visual_bound}. We can see that the object boundaries could be detected in multiple scales through our object perception-enhanced learning.

\section{Results with Different Training Datasets}
\label{sec:differ_train}
In the main experiment, we follow previous methods [13–15, 46] to first pretrain our model on static images for fair comparisons. To study the effects of different training data on the final segmentation results, we additionally conduct experiments to train COLM on DAVIS2017 [50] only, YouTubeVOS2019 only, and a mix of both. The performance comparison with previous methods are shown in Table 5.

\section{Results with Multi-scale Testing}
\label{sec:multiscale_test}
Multi-scale evaluation is a commonly used trick in segmentation tasks [5, 13, 15] to boost the performance by merging the results of inputs under different data augmentations. Here we follow XMem [13] to apply image scaling and vertical mirroring and simply average the output probabilities to obtain the final masks.

\section{Visualization of Reconstruction Attention map and Readout Features}
\label{sec:visual_features}
We visualize the reconstruction attention map(Sec~\ref{subsec:ostmae_branch}) and readout features ($F^M$ in Sec~\ref{subsec:vos_branch}) of the memory-based method~\cite{cheng2022xmem} in Figure 8 to further demonstrate the effectiveness of the proposed Object Perception-enhanced Learning(OPL) strategy.

\section{Implementation Details}
\label{sec:impl_details}

loss weights $\gamma$, $\gamma_1$ and $\gamma_2$ are 1, 0.1 and 0.02
The input image is processed by a random crop of 384 pixels.
We use a batch size of 16 during the static image pretraining stage with each synthetic video containing three augmented frames.
We use a batch size of 8 during main training with each randomly sampling data containing eight frames in chronological order and three potentially existed objects from the same video following~\cite{cheng2022xmem}. The range of sampling changes with the training process: in the intermediate period of training, the sampling range is set larger, while at the end of training, it is set smaller to narrow the gap between training and inference.

By default, we first pretrain on static images for 160K iterations then perform main training for 260K iterations. total training time takes about 4 days.
With a base learning rate of $10^{\5}$, we apply step learning rate decay with a decay ratio of $\nu$ = 0.1.

\section{Rationale}
\label{sec:rationale}
Having the supplementary compiled together with the main paper means that~\cite{bhat2020learning}:
\begin{itemize}
\item The supplementary can back-reference sections of the main paper, for example, we can refer to \cref{sec:intro};
\item The main paper can forward reference sub-sections within the supplementary explicitly (e.g. referring to a particular experiment); 
\item When submitted to arXiv, the supplementary will already included at the end of the paper.
\end{itemize}
To split the supplementary pages from the main paper, you can use \href{https://support.apple.com/en-ca/guide/preview/prvw11793/mac#:~:text=Delete%20a%20page%20from%20a,or%20choose%20Edit%20%3E%20Delete).}{Preview (on macOS)}, \href{https://www.adobe.com/acrobat/how-to/delete-pages-from-pdf.html#:~:text=Choose%20%E2%80%9CTools%E2%80%9D%20%3E%20%E2%80%9COrganize,or%20pages%20from%20the%20file.}{Adobe Acrobat} (on all OSs), as well as \href{https://superuser.com/questions/517986/is-it-possible-to-delete-some-pages-of-a-pdf-document}{command line tools}.
